# Supplementary material for: StaICC: Standardized Evaluation for Classification Task in In-context Learning
Source: arXiv:2501.15708 source file (2025-04-18)
Supplement: Supplementary file 1 [file appendix11.tex]

\appendix

\section{Models and Datasets}
\label{appendix:model_data_cite}

\textbf{We cite the models and datasets involved in this paper here.} 

\paragraph{Models} GPT2 (137M, M: 380M, L: 812M, XL: 1.61B)~\citep{radford2019language}, Pythia~\citep{biderman2023pythia} (14M$\sim$6.9B), OPT~\citep{zhang2022opt} (1.3B, 2.7B, 6.7B), GPT-J~\citep{wang2021gpt} (6B), GPT-NEO (125M, 1.3B, 2.7B)~\citep{gpt-neo}, FALCON (7B, 7B instruction-tuned)~\citep{falcon40b}, Qwen (7B)~\citep{qwen}, QWen2 (7B, 7B instruction-tuned, 72B instruction-tuned)~\citep{qwen2}, and LLaMa2 (7B, 13B, 34B)~\citep{touvron2023llama}. 

\paragraph{Datasets} SST-2~\citep{sst2}, RTE~\citep{RTE1, RTE2, RTE3, RTE5}, AGNews~\citep{Zhang2015CharacterlevelCN}, TREC~\citep{trec1, trec2}, Subjective~\citep{subj}, MR~\citep{MR}, DBPedia~\citep{dbpedia}, SST-5~\citep{sst2}, MRPC~\citep{mrpc}, CommitmentBank~\citep{commitmentbank}, Financial Phrasebank~\citep{FP}.
